# Supplementary material for: Neural Descriptor Fields: SE(3)-Equivariant Object Representations for Manipulation
Source: arXiv:2112.05124 source file (2021-12-09)
Supplement: Supplementary file 1 [file appendix.tex]

\appendix

\setcounter{section}{0}
\setcounter{figure}{0}

\section{Appendix}
\label{sec: appendix}
